# Supplementary material for: MatchNorm: Learning-based Point Cloud Registration for 6D Object Pose Estimation in the Real World
Source: arXiv:2203.15309 source file (2022-08-23)
Supplement: Supplementary file 1 [file 6-supplementary.tex]

\begin{figure}[!ht]
    \centering
    \includegraphics[width=\textwidth]{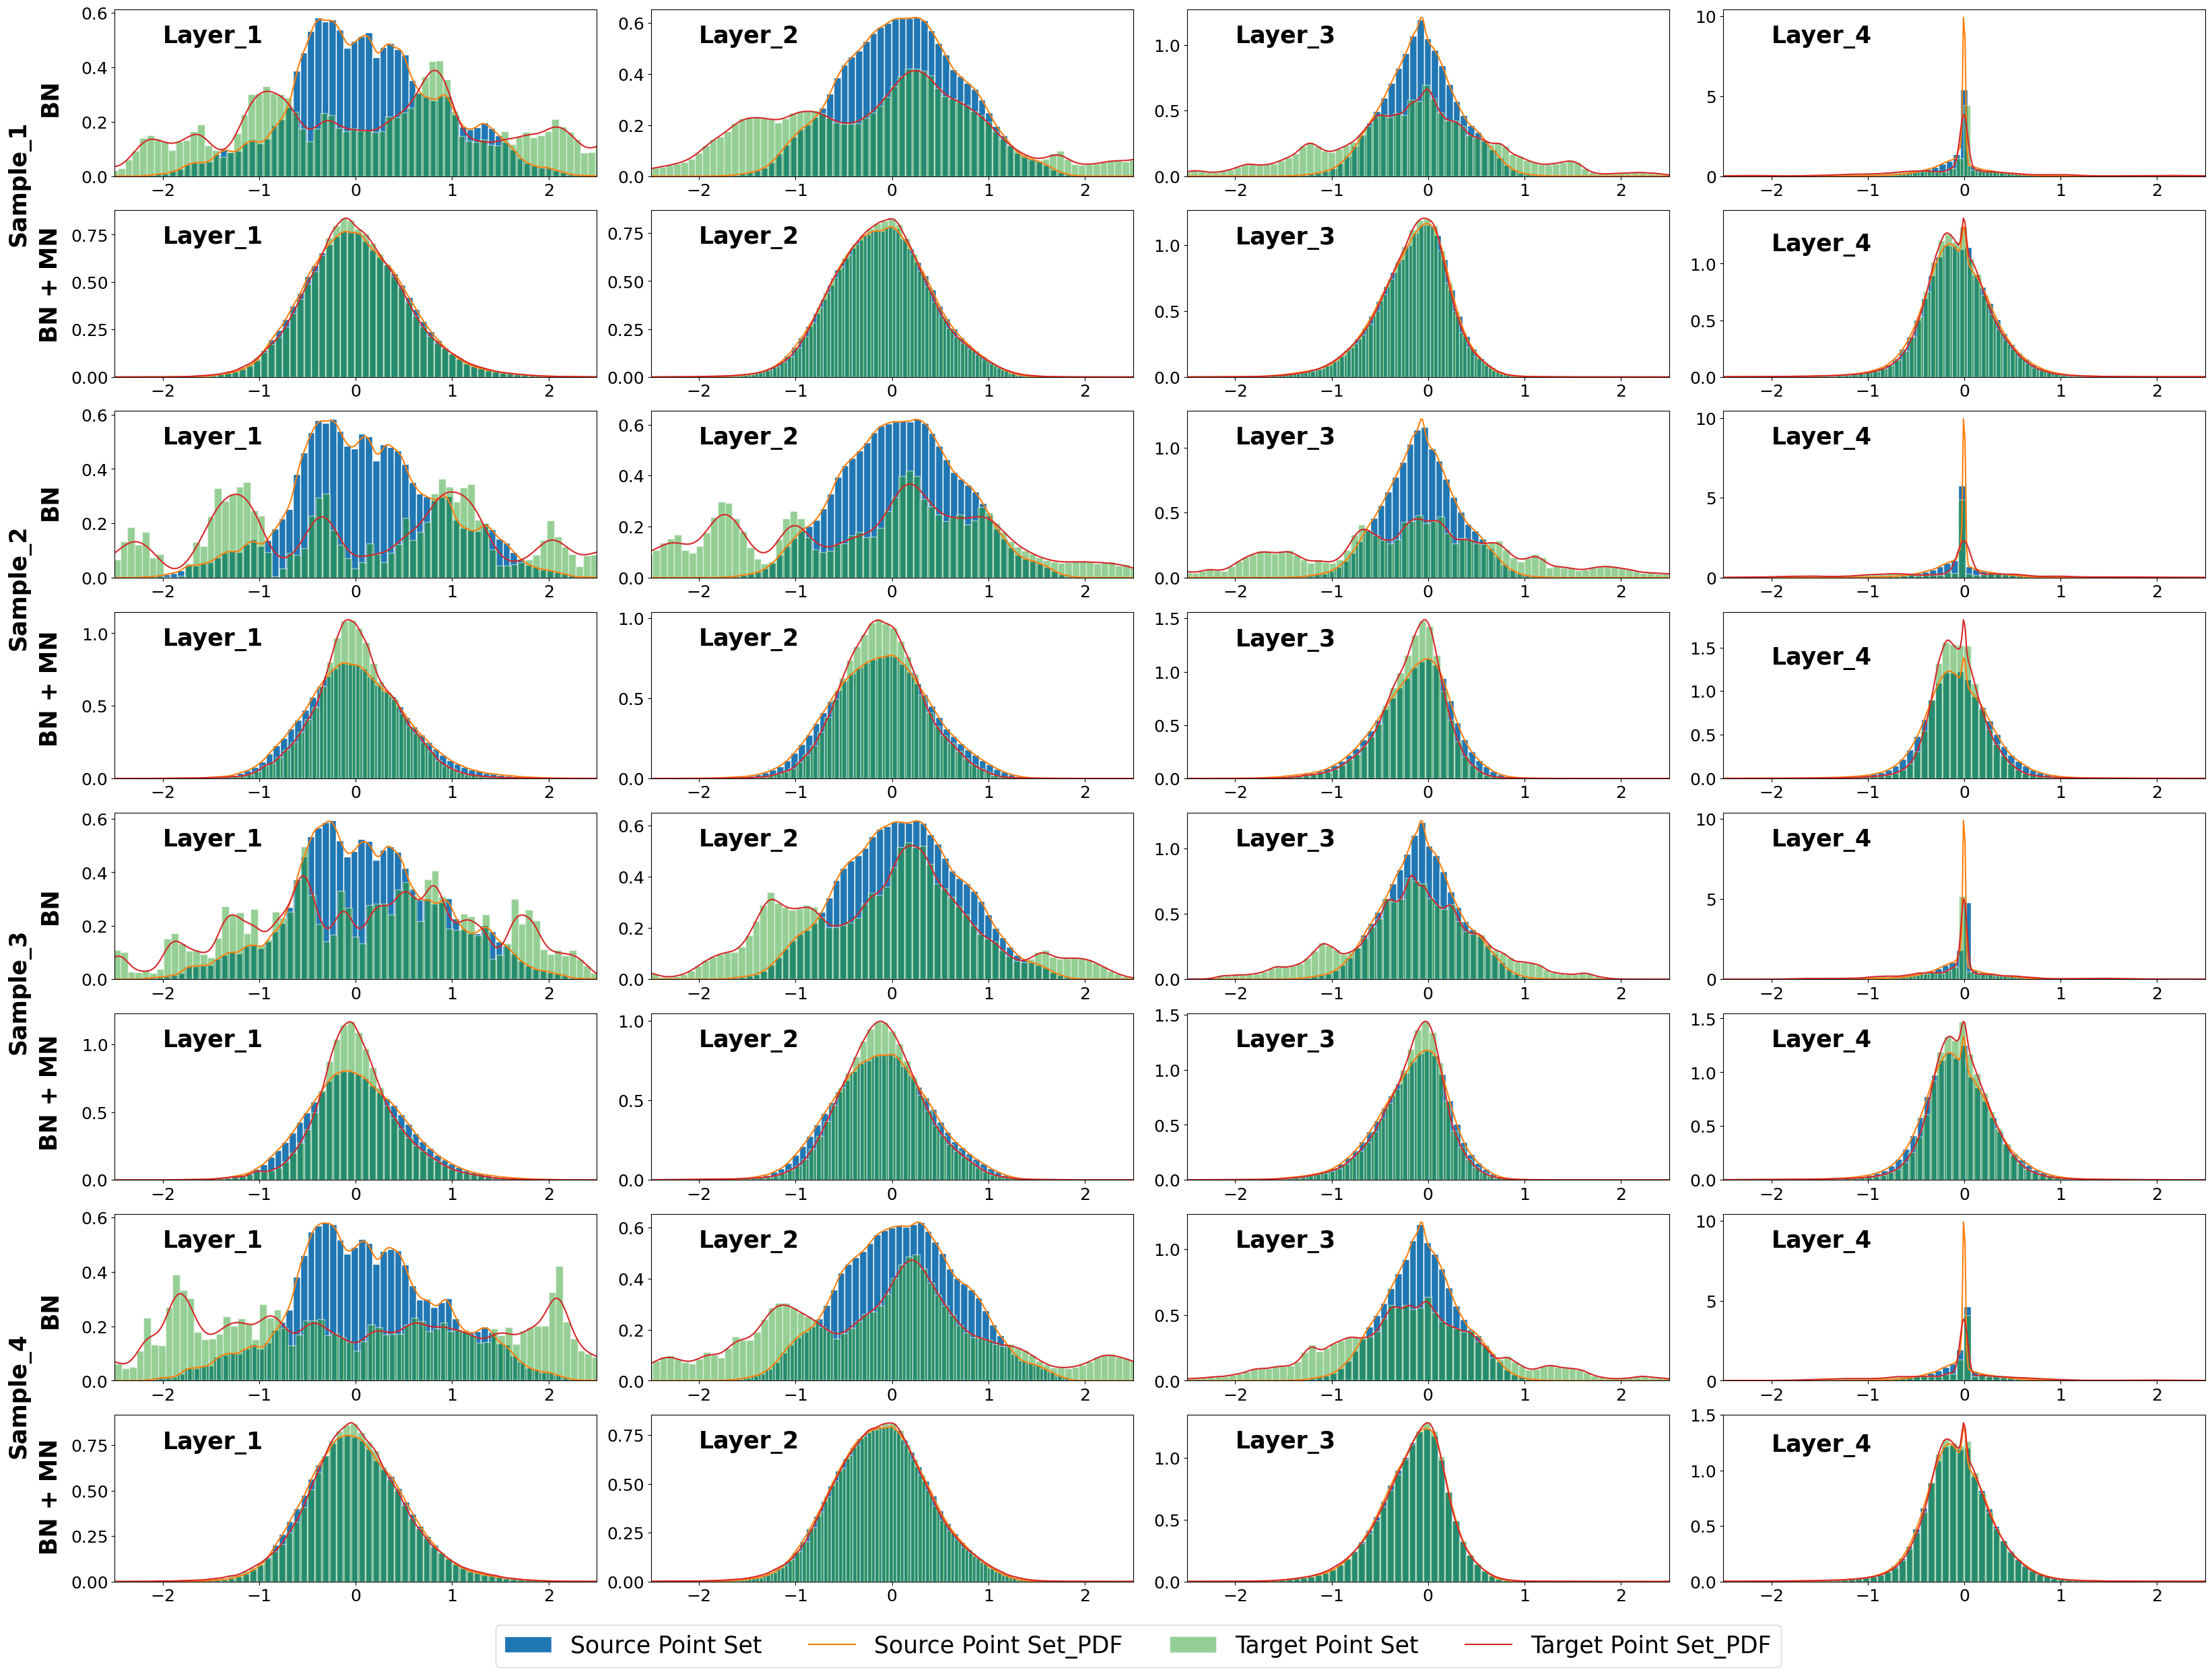}
    \caption{\label{fig:db0} {\bf Feature distributions at different network layers with real-world data.} We show the distribution of the output of the different layer for different samples within one batch, with and without Match Normalization. Match Normalization consistently makes the source and target distributions much more similar.}

\end{figure}

\section{Additional Distribution Visualizations}
As mentioned in Section~3.3 of the main paper, we compare the source and target distributions of all the samples in a batch in~\cref{fig:db0,fig:db1,fig:db2,fig:db3,fig:db4}. When Match Normalization is not used, there is a clear distribution mismatch in every data pair. These differences then affect the number of matched points, ultimately leading to low registration accuracy. Match Normalization makes the distributions of the two point sets much more similar. 

\section{Generalization to New Objects and Across Datasets}
In this experiment, we demonstrate the model's generalization performance obtained with Match Normalization. To this end, we use a model trained on synthetic data and test it on real datasets.
Specifically, for training, we use object mesh models from the ModelNet40 dataset training split. To generate training target point clouds, we exploit Pytorch3D to render the depth map with a randomly given camera pose and intrinsic camera parameters. We use the same parameters as in Section~4.1 to train the model. In the testing phase, we evaluate the resulting model on three real world datasets, TUD-L, LINEMOD and Occluded-LINEMOD, without any fine-tuning. Note that the test objects in these datasets haven't been seen in the training phase. As shown in~\cref{tab:tudl_sup,tab:lm_sup,tab:lmo_sup}, where we also provide the results obtained by training on real data, our model trained on ModelNet40 only (`Ours-DCP+ICP-M') still outperforms Super4PCS and TEASER++. This demonstrates that Match Normalization makes learning-based 3D  object registration applicable to real data while maintaining the ability of point-cloud-based registration to generalize to unseen objects.

\begin{figure}[!ht]
    \centering
    \includegraphics[width=\textwidth]{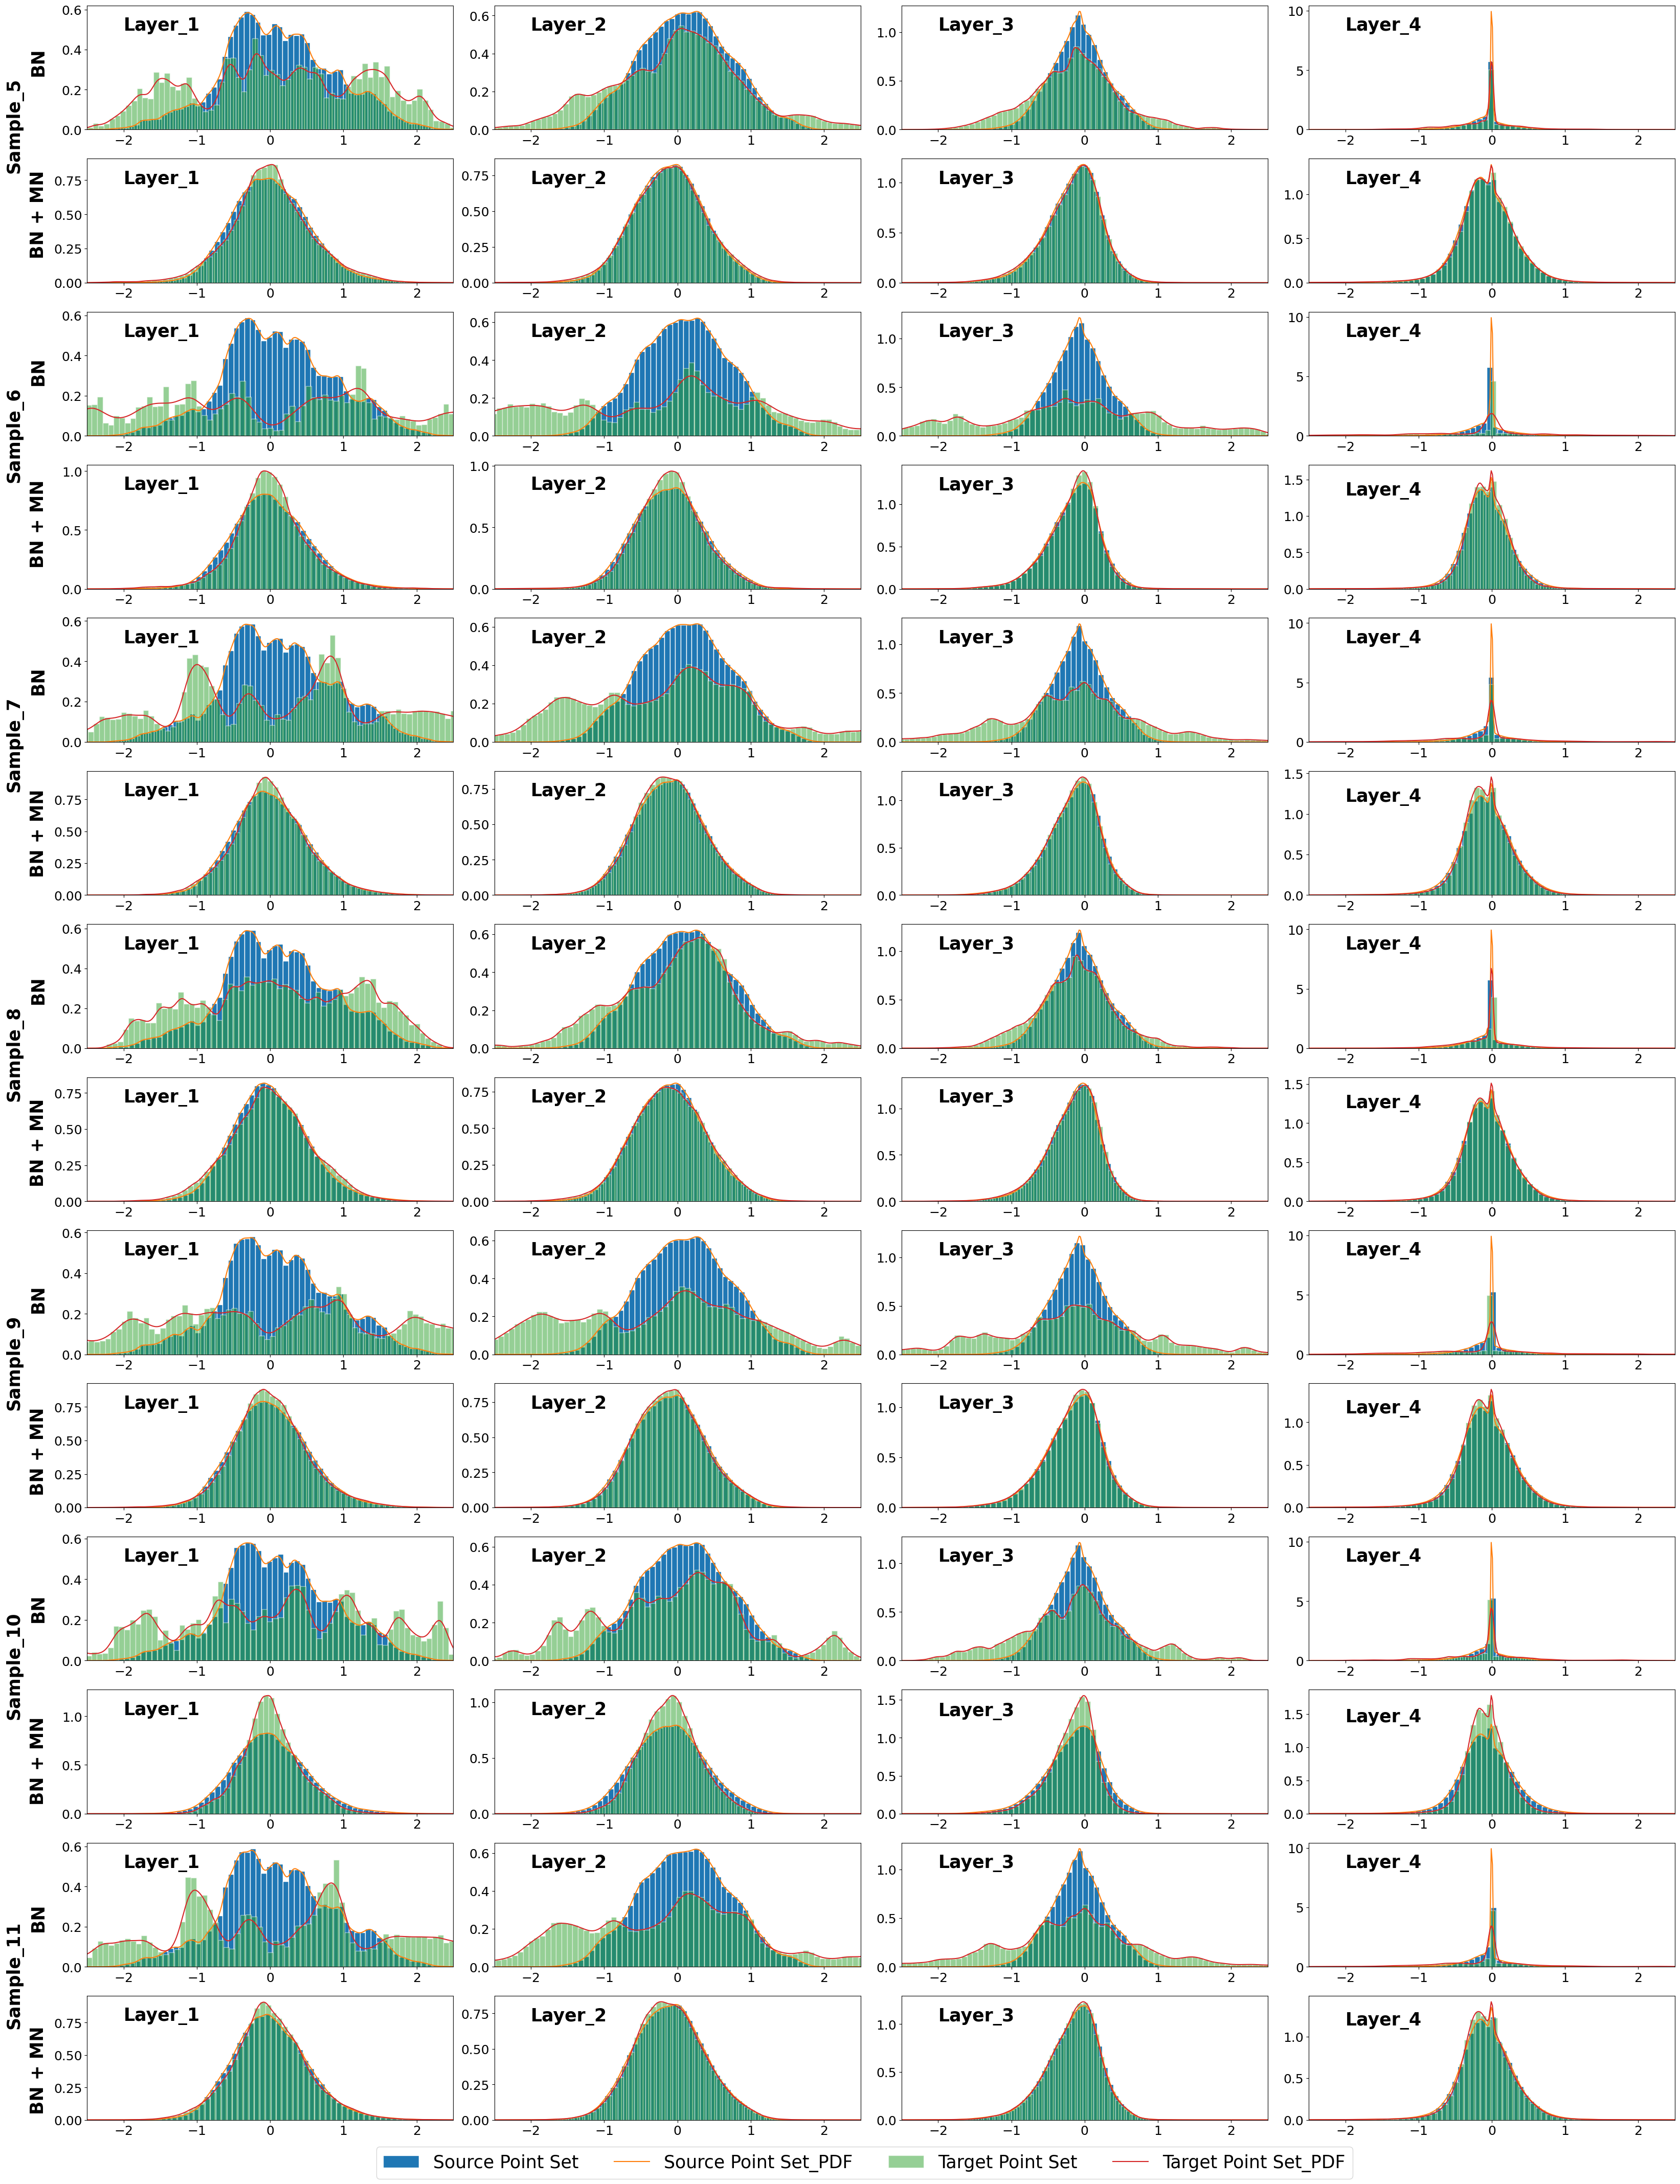}
    \caption{\label{fig:db1} {\bf Feature distributions at different network layers with real-world data.} }

\end{figure}
\begin{figure}[!ht]
    \centering
    \includegraphics[width=\textwidth]{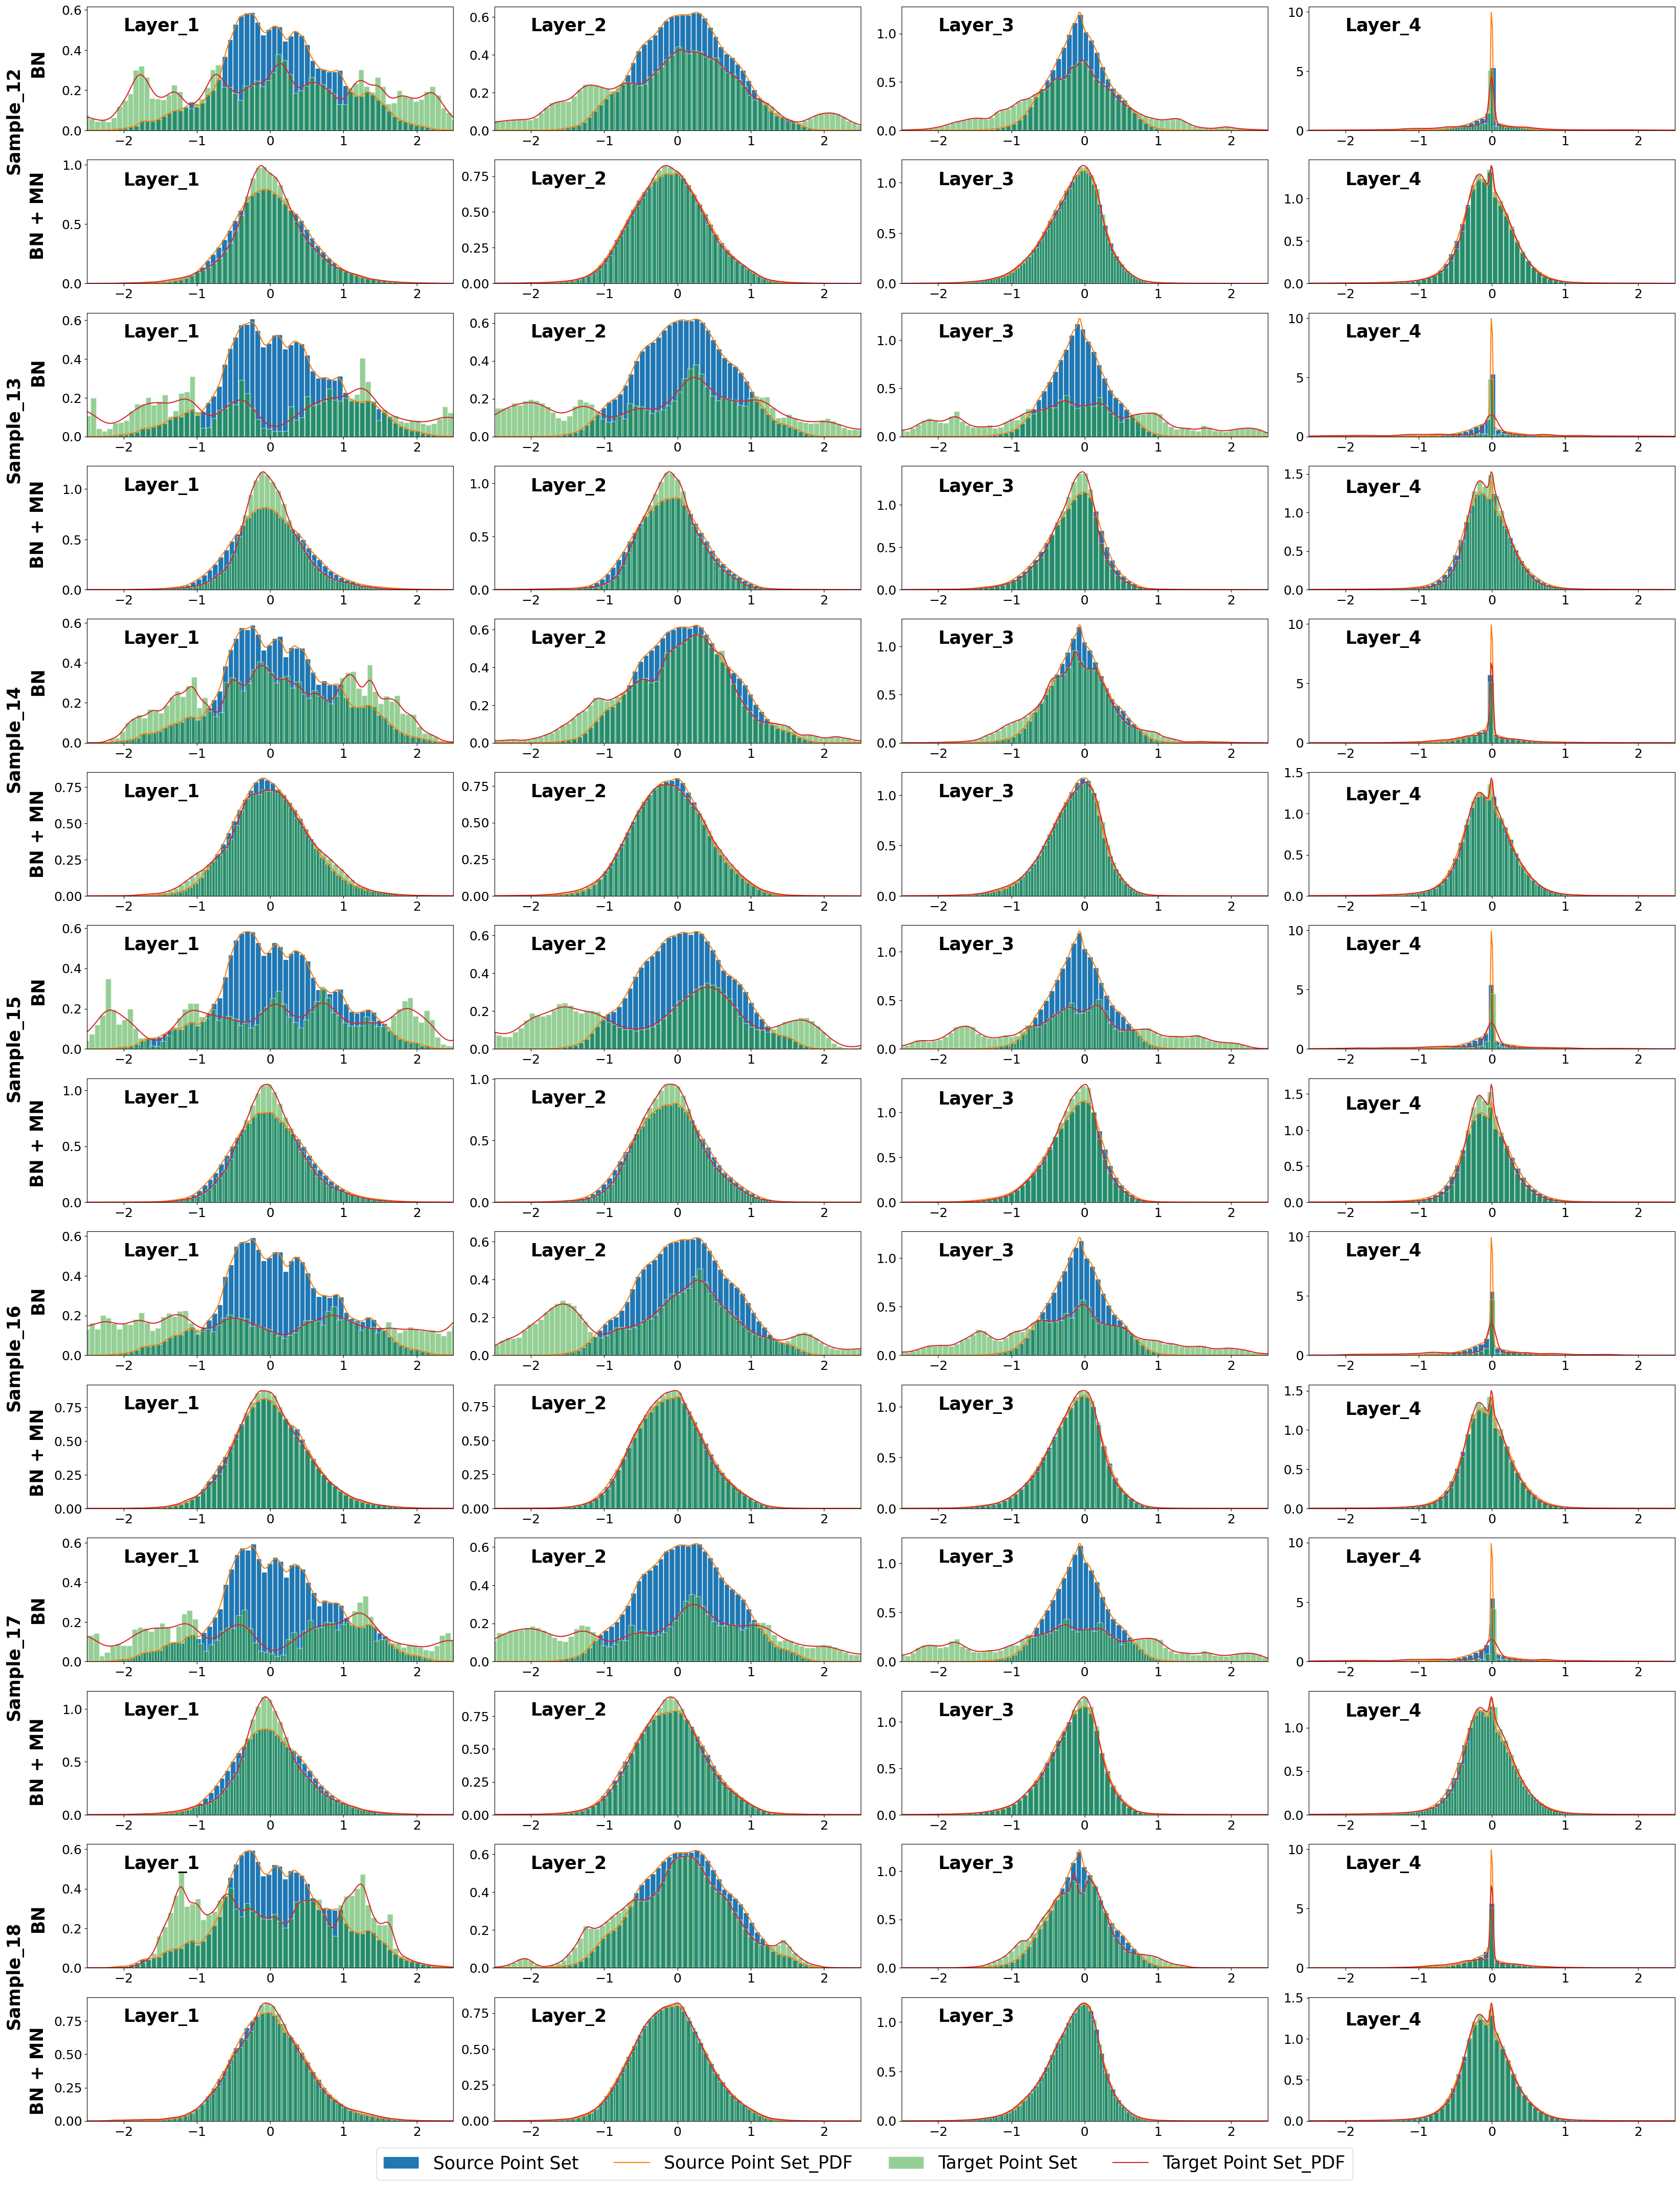}
    \caption{\label{fig:db2} {\bf Feature distributions at different network layers with real-world data.} }
    \vspace{-2em}
\end{figure}
\begin{figure}[!ht]
    \centering
    \includegraphics[width=\textwidth]{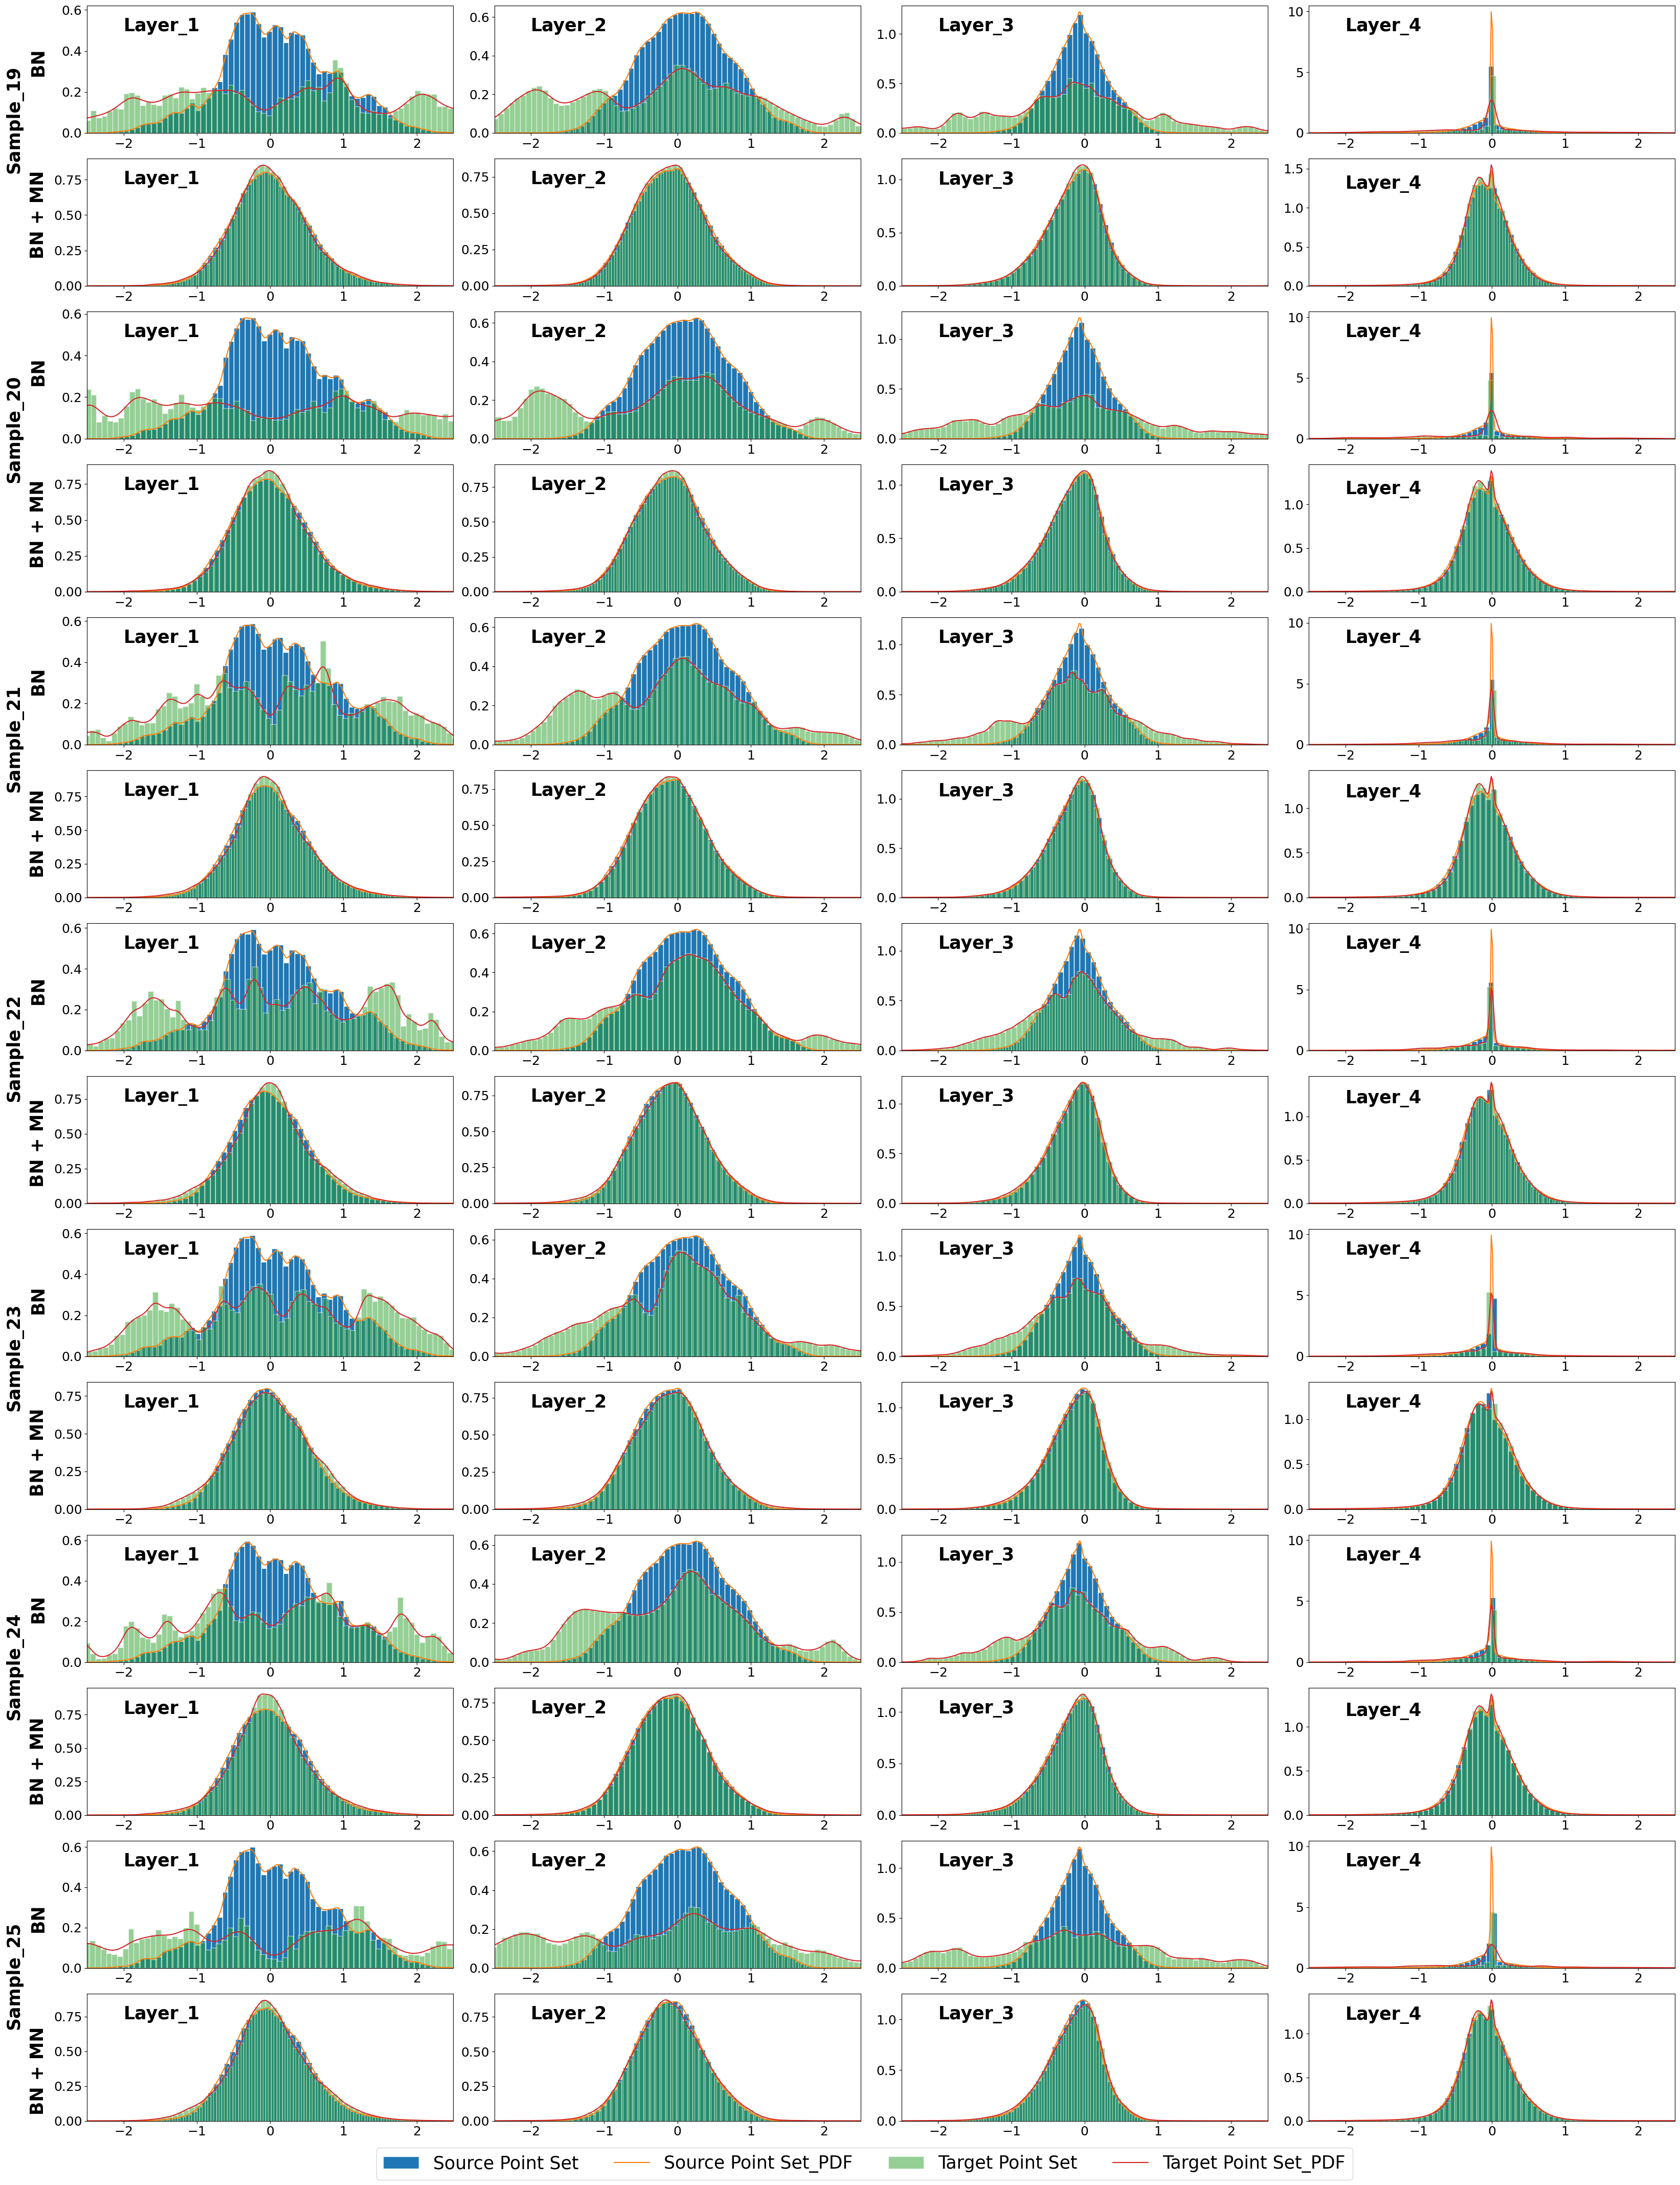}
    \caption{\label{fig:db3} {\bf Feature distributions at different network layers with real-world data.} }
    \vspace{-2em}
\end{figure}
\begin{figure}[!ht]
    \centering
    \includegraphics[width=\textwidth]{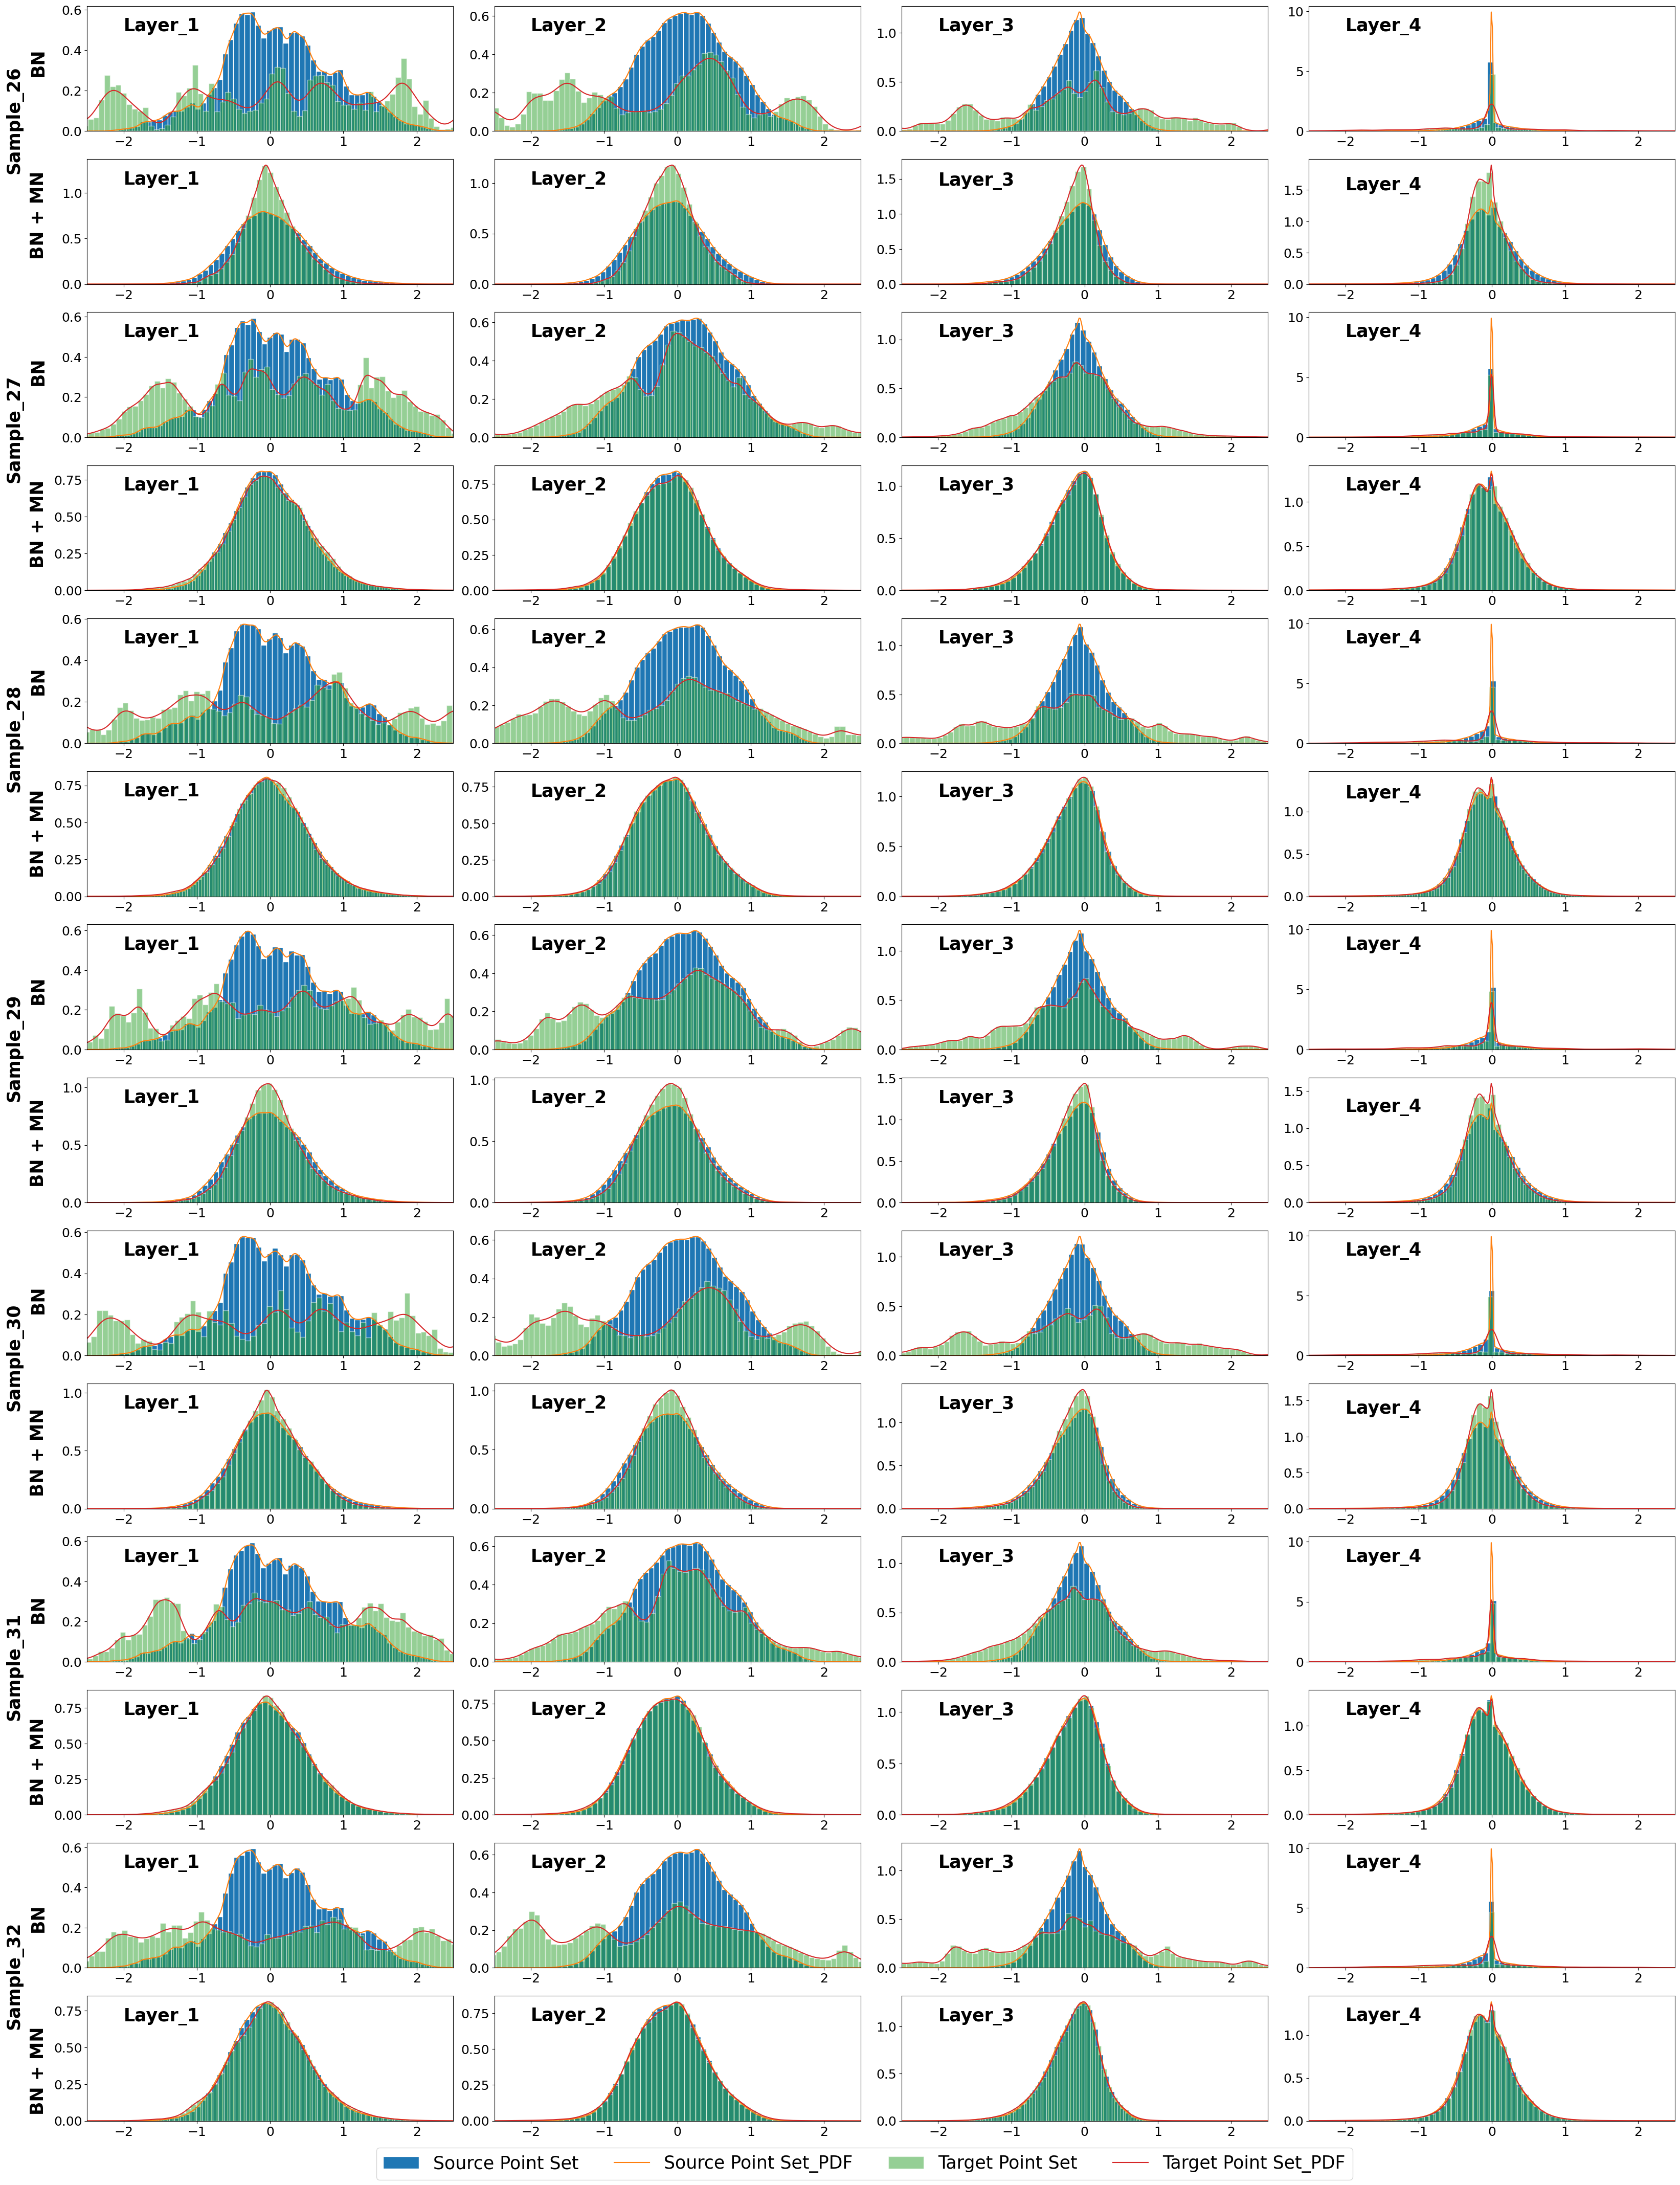}
    \caption{\label{fig:db4} {\bf Feature distributions at different network layers with real-world data.} }
    \vspace{-2em}
\end{figure}

\begin{table*}[!ht]
    \centering
    {\scriptsize
    \setlength{\tabcolsep}{1.mm}{
    \begin{tabular}{l|ccc|ccc|c|cccc}
        \toprule
        & \multicolumn{3}{c|}{Rotation mAP} & \multicolumn{3}{c|}{Translation mAP} & \multicolumn{1}{c|}{ADD} & \multicolumn{4}{c}{BOP Benchmark} \\
        Method & $5^{\circ}$ & $10^{\circ}$ & $20^{\circ}$ & $1cm$ & $2cm$ & $5cm$ & $0.1d$ & VSD & MSSD & MSPD & AR\\
        \midrule
        ICP                 & 0.02 & 0.02 & 0.02 & 0.01 & 0.14 & 0.57 & 0.02 & 0.117 & 0.023 & 0.027 & 0.056 \\
        \rowcolor{tabgray}
        FGR(FPFH)           & 0.00 & 0.01 & 0.01 & 0.04 & 0.25 & 0.63 & 0.01 & 0.071 & 0.007 & 0.008 & 0.029 \\
        TEASER++(FPFH)      & 0.13 & 0.17 & 0.19 & 0.03 & 0.22 & 0.56 & 0.17 & 0.175 & 0.196 & 0.193 & 0.188 \\
        \rowcolor{tabgray}
        Super4PCS           & 0.30 & 0.50 & 0.56 & 0.05 & 0.40 & 0.92 & 0.54 & 0.265 & 0.500 & 0.488 & 0.418 \\
        DCP(v2)             & 0.00 & 0.01 & 0.02 & 0.02 & 0.07 & 0.55 & 0.01 & 0.0253 & 0.051 & 0.039 & 0.038 \\ 
        \rowcolor{tabgray}
        % IDAM(GNN)           & 0.02 & 0.06 & 0.11 & 0.02 & 0.09 & 0.49 & 0.07 & 0.076 & 0.110 & 0.105 & 0.097 \\
        IDAM(FPFH)          & 0.05 & 0.12 & 0.20 & 0.03 & 0.17 & 0.63 & 0.13 & 0.100 & 0.194 & 0.166 & 0.153 \\
        IDAM                & 0.03 & 0.05 & 0.10 & 0.02 & 0.08 & 0.49 & 0.05 & 0.067 & 0.108 & 0.099 & 0.091\\ % IDAM(DGCNN)
        \rowcolor{tabgray}
        $\star$Vidal-Sensors18 & - & - & - & - & - & - & - & 0.811 & 0.910 & 0.907 & 0.876 \\
        $\star$Drost & - & - & - & - & - & - & - & 0.809 & 0.875 & 0.872 & 0.852 \\
        \rowcolor{tabgray}
        Ours-IDAM           & 0.36 & 0.46 & 0.53 & 0.23 & 0.47 & 0.75 & 0.46 & 0.339 & 0.502 & 0.492 & 0.444\\ % IDAM(DGCNN+MN)
        Ours-IDAM+ICP       & 0.56 & 0.58 & 0.61 & 0.55 & 0.66 & 0.81 & 0.58 & 0.580 & 0.604 & 0.618 & 0.601\\ % IDAM(DGCNN+MN+ICP)
        \rowcolor{tabgray}
        Ours-DCP            & 0.70 & 0.81 & 0.87 & 0.71 & 0.86 & 0.97 & 0.85 & 0.700 & 0.853 & 0.852 & 0.801\\
        Ours-DCP+ICP       & \textbf{0.91}& \textbf{0.92}& \textbf{0.93}& \textbf{0.86}& \textbf{0.95}& \textbf{0.99}& \textbf{0.93}& \textbf{0.859} & \textbf{0.914} & \textbf{0.935} & \textbf{0.903}\\
        % Ours-DCP-Modelnet & 0.05 & 0.17 & 0.44 & 0.05 & 0.29 & 0.87 & 0.39 & 0.244 & 0.479 & 0.468 & 0.397 \\
        Ours-DCP+ICP-M & 0.62 & 0.66 & 0.72 & 0.60 & 0.73 & 0.89 & 0.70 & 0.666 & 0.706 & 0.725 & 0.699 \\ 
        \bottomrule
    \end{tabular}
    }}
    \caption{Quantitative comparison of our method with previous work on the \textbf{TUD-L} real scene dataset. The results for Vidal-Sensor18~\cite{Vidal18} and Drost (Drost-CVPR10-3D-Edges)~\cite{Drost10} were directly taken from the BOP leaderboard, and, in contrast with all the other results, were obtained without using a mask for the target point cloud. 
    `Ours-DCP+ICP-M' is the model which trained on the synthetic dataset ModelNet40. Our contributions not only allow existing learning-based methods to successfully register real-world data, but also keep their generalization ability to unseen objects.
    }
    \label{tab:tudl_sup}
    \vspace{-2.25em}
\end{table*}

\begin{table*}[!t]
    \centering
    {\scriptsize
    \setlength{\tabcolsep}{1mm}{
    \begin{tabular}{l|ccc|ccc|c|cccc}
        \toprule
        & \multicolumn{3}{c|}{Rotation mAP} & \multicolumn{3}{c|}{Translation mAP} & \multicolumn{1}{c|}{ADD} & \multicolumn{4}{c}{BOP Benchmark} \\
        Method & $5^{\circ}$ & $10^{\circ}$ & $20^{\circ}$ & $1cm$ & $2cm$ & $5cm$ & $0.1d$ & VSD & MSSD & MSPD & AR\\
        \midrule
        ICP                 & 0.01 & 0.01 & 0.01 & 0.07 & 0.36 & 0.85 & 0.01 & 0.085 & 0.014 & 0.032 & 0.044  \\
        \rowcolor{tabgray}
        FGR(FPFH)           & 0.00 & 0.00 & 0.00 & 0.08 & 0.43 & 0.85 & 0.00 & 0.055 & 0.000 & 0.009 & 0.021  \\
        TEASER++(FPFH)      & 0.01 & 0.02 & 0.05 & 0.04 & 0.26 & 0.77 & 0.02 & 0.096 & 0.060 & 0.093 & 0.083  \\
        \rowcolor{tabgray}
        Super4PCS           & 0.01 & 0.03 & 0.06 & 0.06 & 0.31 & 0.83 & 0.03 & 0.054 & 0.072 & 0.113 & 0.080 \\
        DCP(v2)             & 0.00 & 0.00 & 0.01 & 0.03 & 0.30 & 0.83 & 0.00 & 0.055 & 0.018 & 0.059 & 0.044 \\ 
        % \rowcolor{tabgray}
        % % IDAM(GNN)           & 0.02 & 0.06 & 0.11 & 0.02 & 0.09 & 0.49 & 0.07 & 0.076 & 0.110 & 0.105 & 0.097 \\
        \rowcolor{tabgray}
        IDAM(FPFH)          & 0.00 & 0.00 & 0.02 & 0.04 & 0.18 & 0.73 & 0.00 & 0.044 & 0.033 & 0.066 & 0.048 \\
        IDAM                & 0.00 & 0.02 & 0.06 & 0.07 & 0.26 & 0.76 & 0.02 & 0.063 & 0.088 & 0.119 & 0.090 \\ % IDAM(DGCNN) /home/hush/projects/idam/ckpt/0304_train_DGCNNdcp_lm/models/model.4.t7 /home/hush/projects/idam/0305idamDGCNNdcp_lmo-test.csv
        \rowcolor{tabgray}
        $\star$Vidal-Sensors18 & - & - & - & - & - & - & - & 0.473 & 0.625 & 0.647 & 0.582 \\
        $\star$PPF\_3D\_ICP & - & - & - & - & - & - & - & \textbf{0.523} & \textbf{0.669} & \textbf{0.716} & \textbf{0.636} \\
        \rowcolor{tabgray}
        Ours-IDAM            & 0.02 & 0.08 & 0.18 & 0.15 & 0.44 & 0.84 & 0.12 & 0.155 & 0.204 & 0.248 & 0.202 \\ % IDAM(DGCNN+MN) /home/hush/projects/idam/ckpt/0304_train_DGCNN_lm/models/model.3.t7 /home/hush/projects/idam/0305idamDGCNN_lmo-test.csv
        Ours-IDAM+ICP        & 0.15 & 0.22 & 0.32 & 0.23 & 0.58 & 0.88 & 0.25 & 0.349 & 0.320 & 0.374 & 0.348 \\ % IDAM(DGCNN+MN+ICP) /home/hush/projects/idam/ckpt/0304_train_DGCNN_lm/models/model.3.t7 /home/hush/projects/idam/0305idamDGCNNicp_lmo-test.csv
        \rowcolor{tabgray}
        Ours-DCP                & 0.07 & 0.19 & 0.36 & 0.24 & 0.57 & 0.88 & 0.28 & 0.263 & 0.384 & 0.450 & 0.365 \\
        Ours-DCP+ICP          & \textbf{0.31} & \textbf{0.46} & \textbf{0.56} & \textbf{0.37} & \textbf{0.70} & \textbf{0.91} & \textbf{0.47} & 0.478 & 0.542 & 0.612 & 0.544 \\
        % Ours-DCP-Modelnet & 0.01 & 0.04 & 0.14 & 0.09 & 0.39 & 0.84 & 0.06 & 0.138 & 0.186 & 0.256 & 0.193 \\
        Ours-DCP+ICP-M & 0.18 & 0.25 & 0.32 & 0.26 & 0.57 & 0.86 & 0.27 & 0.343 & 0.328 & 0.393 & 0.354 \\
        \bottomrule
    \end{tabular}
    }}
    \caption{Quantitative comparison of our method with previous work on the \textbf{Occluded-LINEMOD} real scene dataset. Vidal-Sensors18~\cite{Vidal18} and PPF\_3D\_ICP~\cite{Drost10} are traditional methods and represent the best depth-only performers from the BOP leaderboard.}
    \label{tab:lmo_sup}
    \vspace{-2.5em}
\end{table*}

\begin{table*}[!t]
    \centering
    {\scriptsize
    \setlength{\tabcolsep}{1mm}{
    \begin{tabular}{l|ccc|ccc|c|cccc}
        \toprule
        & \multicolumn{3}{c|}{Rotation mAP} & \multicolumn{3}{c|}{Translation mAP} & \multicolumn{1}{c|}{ADD} & \multicolumn{4}{c}{BOP Benchmark} \\
        Method & $5^{\circ}$ & $10^{\circ}$ & $20^{\circ}$ & $1cm$ & $2cm$ & $5cm$ & $0.1d$ & VSD & MSSD & MSPD & AR\\
        \midrule
        ICP                 & 0.00 & 0.01 & 0.01 & 0.04 & 0.27 & 0.82 & 0.01 & 0.092 & 0.014 & 0.027 & 0.044 \\
        \rowcolor{tabgray}
        FGR(FPFH)           & 0.00 & 0.00 & 0.00 & 0.05 & 0.31 & 0.89 & 0.00 & 0.068 & 0.000 & 0.010 & 0.026 \\
        TEASER++(FPFH)      & 0.01 & 0.03 & 0.05 & 0.03 & 0.21 & 0.73 & 0.03 & 0.108 & 0.076 & 0.098 & 0.094 \\
        \rowcolor{tabgray}
        Super4PCS           & 0.02 & 0.09 & 0.15 & 0.04 & 0.31 & 0.89 & 0.10 & 0.117 & 0.178 & 0.201 & 0.165 \\
        DCP(v2)             & 0.00 & 0.00 & 0.01 & 0.05 & 0.24 & 0.83 & 0.00 & 0.057 & 0.025 & 0.049 & 0.044 \\ 
        % % IDAM(GNN)           & 0.02 & 0.06 & 0.11 & 0.02 & 0.09 & 0.49 & 0.07 & 0.076 & 0.110 & 0.105 & 0.097 \\
        \rowcolor{tabgray}
        IDAM(FPFH)          & 0.00 & 0.01 & 0.03 & 0.03 & 0.16 & 0.67 & 0.01 & 0.053 & 0.055 & 0.069 & 0.059 \\
        IDAM                & 0.00 & 0.01 & 0.05 & 0.03 & 0.16 & 0.71 & 0.02 & 0.050 & 0.070 & 0.081 & 0.067 \\ % IDAM(DGCNN) /home/hush/projects/idam/ckpt/0304_train_DGCNNdcp_lm/models/model.4.t7  /home/hush/projects/idam/0305idamDGCNNdcp_lm-test.csv
        \rowcolor{tabgray}
        $\star$PPF\_3D\_ICP & - & - & - & - & - & - & - & \textbf{0.719} & \textbf{0.856} & \textbf{0.866} & \textbf{0.814} \\ 
        $\star$Drost & - & - & - & - & - & - & - & 0.678 & 0.786 & 0.789 & 0.751 \\
        \rowcolor{tabgray}
        Ours-IDAM            & 0.01 & 0.07 & 0.15 & 0.13 & 0.38 & 0.87 & 0.11 & 0.148 & 0.194 & 0.209 & 0.184 \\ % IDAM(DGCNN+MN) /home/hush/projects/idam/ckpt/0304_train_DGCNN_lm/models/model.3.t7 /home/hush/projects/idam/0305idamDGCNN_lm-test.csv
        Ours-IDAM+ICP        & 0.15 & 0.23 & 0.27 & 0.25 & 0.54 & 0.91 & 0.23 & 0.352 & 0.311 & 0.345 & 0.336 \\ % IDAM(DGCNN+MN+ICP) /home/hush/projects/idam/ckpt/0304_train_DGCNN_lm/models/model.3.t7 /home/hush/projects/idam/0305idamDGCNNicp_lm-test.csv
        \rowcolor{tabgray}
        Ours-DCP            & 0.10 & 0.27 & 0.49 & 0.26 & 0.60 & 0.95 & 0.37 & 0.319 & 0.490 & 0.529 & 0.446 \\
        Ours-DCP+ICP        & \textbf{0.43} & \textbf{0.59} & \textbf{0.67} & \textbf{0.49} & \textbf{0.83} & \textbf{0.97} & \textbf{0.60} & 0.616 & 0.680 & 0.737 & 0.678 \\
        % Ours-DCP-Modelnet & 0.01 & 0.06 & 0.18 & 0.07 & 0.40 & 0.91 & 0.09 & 0.175 & 0.244 & 0.297 & 0.239 \\
        Ours-DCP+ICP-M & 0.25 & 0.35 & 0.42 & 0.34 & 0.66 & 0.93 & 0.36 & 0.449 & 0.446 & 0.499 & 0.465 \\  
        
        \bottomrule
    \end{tabular}
    }}
    \caption{Quantitative comparison of our method with previous work on the \textbf{LINEMOD} real scene dataset. PPF\_3D\_ICP~\cite{Drost10} and Drost (Drost-CVPR10-3D-Only)~\cite{Drost10} are traditional methods and represent the best depth-only performers from the BOP leaderboard.}
    \label{tab:lm_sup}
    \vspace{-1.25em}
\end{table*}
